# Supplementary material for: CUF: Continuous Upsampling Filters
Source: arXiv:2210.06965 source file (2022-10-20)
Supplement: Supplementary file 1 [file 6_appendix.tex]

\appendix
